# Supplementary material for: Class Impression for Data-free Incremental Learning
Source: arXiv:2207.00005 source file (2022-07-04)
Supplement: Supplementary file 1 [file appendix.tex]

% \section{Supplementary}

\section{Dataset Details}
\label{app_data}

\begin{table*}[h]
\centering
\begin{tabular}{|c|c||c|c|}
\hline
\textbf{View}              & \textbf{\# of cines}    & \textbf{View}              & \textbf{\# of cines}    \\ \hline
A2C   & 1928 & PLAX   & 2747 \\ \hline
A3C & 2095   & PSA   & 2126                  \\ \hline
A4C & 2166   & ---   & ---                  \\ \hline 
\end{tabular}
\caption{ Number of data points for each echo view class.}
\label{tab_arch1}
\end{table*}

\section{Detailed model hyper-parameters}

\begin{table*}[h]
\centering
\begin{tabular}{|c|c|c|c|c|c|}
\hline
\multirow{2}{*}{\textbf{Stage}} & \multirow{2}{*}{\textbf{Hyper-parameters}}          & \multicolumn{4}{|c|}{\textbf{Phase}}    \\
\cline{3-6}
 & & 1   & 2 & 3 & 4 \\
\cline{1-6}
\multirow{6}{*}{\textbf{Synthesize}} & Weight for batch normalization regularization  & --- & 0.2   & 1 & 5 \\ \cline{2-6}
& Weight for total variation L2 regularization & ---   & 0.001  & 0.01  & 0.01                 \\ \cline{2-6}
& Weight for total regularization loss & ---   & 0.01   & 0.1  & 0.001                 \\\cline{2-6}
& Learning rate & ---   & 0.25  & 0.05  & 0.005                 \\\cline{2-6}
& Beta 2 for ADAM optimizer & ---   & 0.09   & 0.9  & 0.009                 \\\cline{2-6}
& Batch size & ---   & 40   & 40  & 40                 \\\hline 

\multirow{7}{*}{\textbf{Train}} & Temporature for distialltion loss  & --- & 2   & 2 & 2 \\ \cline{2-6}
& Weight for distialltion loss & ---   & 5   & 5 & 5                 \\ \cline{2-6}
& Distance for margin loss & ---   & 0.7  & 0.3 & 0.3                 \\ \cline{2-6}
& Weight for margin loss & ---   & 1  & 1 & 1                 
\\ \cline{2-6}
& Temporature for updating centroids of contrastive loss & ---   & 0.99 & 0.99 & 0.99                \\\cline{2-6}

& Learning rate & 0.01   & 0.01   & 0.01 & 0.01                 \\ \cline{2-6}
& Batch size & 40   & 40   & 40 & 40                 \\  \hline 
\end{tabular}
\caption{ Hyper-parameters used for training.}
\label{tab_arch1}
\end{table*}

\section{Visualization of data}

\begin{figure}[h]
\floatsetup{valign=t, heightadjust=all}
	\centering
\begin{subfigure}[t]{\textwidth}
    	\centering
         \begin{subfigure}[t]{0.45\textwidth}
        	\includegraphics[width=1\textwidth]{figures/original_images.pdf}
        	\caption{}
        % 	\caption{Comparison with baselines of class-incremental learning on Heart Echo Dataset}
        	\label{fig:baseline}
        \end{subfigure}
        \hfill
        \begin{subfigure}[t]{0.45\textwidth}
        	\includegraphics[width=1\textwidth]{figures/mean_images.pdf}
        	 \caption{}
            % \caption{Comparison with different configurations on Heart Echo Dataset}
            \label{fig:abalation}
        \end{subfigure}
        \hfill
        \begin{subfigure}[t]{0.45\textwidth}
        	\includegraphics[width=1\textwidth]{figures/my_gen.pdf}
        	 \caption{}
            % \caption{Comparison with different configurations on Heart Echo Dataset}
            \label{fig:abalation}
        \end{subfigure}
        \hfill
        \begin{subfigure}[t]{0.45\textwidth}
        	\includegraphics[width=1\textwidth]{figures/dream_gen.pdf}
        	 \caption{}
            % \caption{Comparison with different configurations on Heart Echo Dataset}
            \label{fig:abalation}
        \end{subfigure}
        \hfill
    	
	\end{subfigure}
	\caption{ (a) Original images from 4 different view classes (A2C,A3C,A4C, and PLAX). (b) Mean images of each class used  for initialization. (c) Synthesized images by \ours (d) Synthesized images by Always Be Dreaming (ABD) [22].
	%in a five-way classification without class-incremental setting. 
}
	\label{compare_table}
\end{figure}

% \begin{table*}[h]
% \centering
% \begin{tabular}{c|c}
% \toprule
% \textbf{Layer}              & \textbf{Details}    \\ \midrule  
% 1   & Dropout($p$ = 0.1)  \\ \hline
% 2 & G-conv($D$, 256) + ELU                     \\ \hline
% 3 & G-conv(256, 64) + ELU                     \\ \hline
% 4 &  FC(64, 1)  +Sigmoid                     \\ \hline
% 5  & Random-vector(4)  \\ \hline
% 6 & Linear(68, 128) + ReLU+BN(128)                   \\ \hline
% 7 & Linear(128, 256)  + ReLU+BN(256)                   \\ \hline
% 8 & FC(256, $D$) +   tanh                  \\ \hline
% 9 & Linear($D$, 32)  ReLU                   \\ \hline     
% 10 & FC(32, 2)                 \\ \bottomrule  
% \end{tabular}
% \caption{ Network architecture of the missing node generator.}
% \label{tab_arch1}
% \end{table*}
